# Supplementary material for: Mining Path Association Rules in Large Property Graphs (with Appendix)
Source: arXiv:2408.02029 source file (2024-09-20)
Supplement: Supplementary file 1 [file 99-supplimetary.tex]

%%
%% This is file `sample-manuscript.tex',
%% generated with the docstrip utility.
%%
%% The original source files were:
%%
%% samples.dtx  (with options: `manuscript')
%% 
%% IMPORTANT NOTICE:
%% 
%% For the copyright see the source file.
%% 
%% Any modified versions of this file must be renamed
%% with new filenames distinct from sample-manuscript.tex.
%% 
%% For distribution of the original source see the terms
%% for copying and modification in the file samples.dtx.
%% 
%% This generated file may be distributed as long as the
%% original source files, as listed above, are part of the
%% same distribution. (The sources need not necessarily be
%% in the same archive or directory.)
%%
%% The first command in your LaTeX source must be the \documentclass command.
%%%% Small single column format, used for CIE, CSUR, DTRAP, JACM, JDIQ, JEA, JERIC, JETC, PACMCGIT, TAAS, TACCESS, TACO, TALG, TALLIP (formerly TALIP), TCPS, TDSCI, TEAC, TECS, TELO, THRI, TIIS, TIOT, TISSEC, TIST, TKDD, TMIS, TOCE, TOCHI, TOCL, TOCS, TOCT, TODAES, TODS, TOIS, TOIT, TOMACS, TOMM (formerly TOMCCAP), TOMPECS, TOMS, TOPC, TOPLAS, TOPS, TOS, TOSEM, TOSN, TQC, TRETS, TSAS, TSC, TSLP, TWEB.
% \documentclass[acmsmall]{acmart}

%%%% Large single column format, used for IMWUT, JOCCH, PACMPL, POMACS, TAP, PACMHCI
% \documentclass[acmlarge,screen]{acmart}

%%%% Large double column format, used for TOG
% \documentclass[acmtog, authorversion]{acmart}

%%%% Generic manuscript mode, required for submission
%%%% and peer review
\documentclass[sigconf,anonymous]{acmart}

\usepackage[ruled, vlined, linesnumbered]{algorithm2e}
\usepackage{algorithmic}
\usepackage{subfig}
\usepackage{epsfig}
\newcommand{\graph}{\ensuremath{\mathcal{G}}}
\newcommand{\edges}{\ensuremath{\mathcal{E}}}
\newcommand{\vertices}{\ensuremath{\mathcal{V}}}
\newcommand{\elabel}{\ensuremath{\ell}}
\newcommand{\elabels}{\ensuremath{\mathcal{L}}}
\newcommand{\attributes}{\ensuremath{\mathcal{A}}}
\newcommand{\rules}{\ensuremath{\mathcal{R}}}

\newcommand{\pathpatterns}{\ensuremath{\mathcal{P}}}
\newcommand{\minsup}{\ensuremath{\theta}}

\newcommand{\candidates}{\ensuremath{\mathcal{C}}}

% \newcommand{\histories}{\ensuremath{\mathcal{H}}}
% \newcommand{\classes}{\ensuremath{\mathcal{C}}}

% \newcommand{\paths}{\ensuremath{\mathcal{P}}}
% \newcommand{\vocab}{\ensuremath{\elabels}}
% \newcommand{\PA}{\ensuremath{PA}}
% \newcommand{\CPQ}{{\em CPQ}}
% \newcommand{\cpq}{\ensuremath{CPQ}}
% \newcommand{\RQ}{\ensuremath{RQ}}
% \newcommand{\degreesum}[2]{d^{#1}_{#2}}

%%
%% \BibTeX command to typeset BibTeX logo in the docs
\AtBeginDocument{%
  \providecommand\BibTeX{{%
    \normalfont B\kern-0.5em{\scshape i\kern-0.25em b}\kern-0.8em\TeX}}}

%% Rights management information.  This information is sent to you
%% when you complete the rights form.  These commands have SAMPLE
%% values in them; it is your responsibility as an author to replace
%% the commands and values with those provided to you when you
%% complete the rights form.
% \setcopyright{acmcopyright}
% \copyrightyear{2018}
% \acmYear{2018}
% \acmDOI{10.1145/1122445.1122456}

% %% These commands are for a PROCEEDINGS abstract or paper.
% \acmConference[Woodstock '18]{Woodstock '18: ACM Symposium on Neural
%   Gaze Detection}{June 03--05, 2018}{Woodstock, NY}
% \acmBooktitle{Woodstock '18: ACM Symposium on Neural Gaze Detection,
%   June 03--05, 2018, Woodstock, NY}
% \acmPrice{15.00}
% \acmISBN{978-1-4503-XXXX-X/18/06}

%%
%% Submission ID.
%% Use this when submitting an article to a sponsored event. You'll
%% receive a unique submission ID from the organizers
%% of the event, and this ID should be used as the parameter to this command.
%%\acmSubmissionID{123-A56-BU3}

%%
%% The majority of ACM publications use numbered citations and
%% references.  The command \citestyle{authoryear} switches to the
%% "author year" style.
%%
%% If you are preparing content for an event
%% sponsored by ACM SIGGRAPH, you must use the "author year" style of
%% citations and references.
%% Uncommenting
%% the next command will enable that style.
%%\citestyle{acmauthoryear}

%%
%% end of the preamble, start of the body of the document source.
\begin{document}

%%
%% The "title" command has an optional parameter,
%% allowing the author to define a "short title" to be used in page headers.
\title{Path Association Rule Mining}

%%
%% The "author" command and its associated commands are used to define
%% the authors and their affiliations.
%% Of note is the shared affiliation of the first two authors, and the
%% "authornote" and "authornotemark" commands
%% used to denote shared contribution to the research.
\author{Yuya Sasaki}
\email{sasaki@ist.osaka-u.ac.jp}
\affiliation{%
  \institution{Osaka University}
}

\newtheorem{property}{Property}[section]
%\newtheorem{lemma}{Lemma}[section]
%\newtheorem{corollary}{Corollary}[section]
%\newtheorem{example}{Example}[section]
%\newtheorem{proposition}{Proposition}[section]

%%
%% By default, the full list of authors will be used in the page
%% headers. Often, this list is too long, and will overlap
%% other information printed in the page headers. This command allows
%% the author to define a more concise list
%% of authors' names for this purpose.
\renewcommand{\shortauthors}{Trovato and Tobin, et al.}

\maketitle

\appendix
\section{Proof}
We show proofs of our theorems and lemmas in the main body.

\smallskip
\smallskip
{\sc Theorem} 3.1. 
{\it If path pattern $p \subseteq p'$, $\vertices(p) \supseteq \vertices(p')$.}
\smallskip
%\end{theorem}

{\it Proof}: When $p$ is dominated by $p'$, $p$ is not longer than $p'$, all edge labels on $p$ and $p'$ are the same order, and attribute sets on $p$ are subset or equal to those on $p'$.
All vertices that match $p'$ are matched with path patterns whose attributes are subset of $p'$.
Therefore, if path pattern $p \subseteq p'$, $\vertices(p) \supseteq \vertices(p')$.
\hfill{} $\square$

\smallskip
{\sc Lemma} 3.2. 
{\it If prefix of path patterns is not frequent, the whole path patterns are not frequent.}
\smallskip

{\it Proof}: If $v$ matches $p=(A_0, \elabel_1, \cdots, \elabel_{n}, A_m)$, $v$ matches $(A_0, \elabel_1, \cdots,$ $\elabel_{n}, A_m)$ where $m < n$.
Similarly, if  $v$ does note match $(A_0, \elabel_1, \cdots,$ $\elabel_{m}, A_m)$, $v$ does not matches $(A_0, \elabel_1, \cdots, \elabel_{n}, A_n)$.
Therefore, if prefix of path patterns is not frequent, the whole path patterns are not frequent.
\hfill{} $\square$

\smallskip
{\sc Lemma} 3.3. 
{\it If path pattern $p$ is not frequent, $p'$ such that $\forall A_i' \supseteq A_i$ and $\elabel_i = \elabel'_i$ is not frequent.}
\smallskip

{\it Proof}: If $v$ matches $p'$, $v$ matches $p$ because $p'$ is more complex than $p$.
Similarly, if  $v$ does note match $p$, $v$ does not matches $p'$.
Therefore, if $p$ is not frequent, $p'$ is not frequent.
\hfill{} $\square$

\smallskip
{\sc Lemma} 3.5. 
{\it Given length $n$ and $(\elabel_{n}, A_n)$, the maximum number of matched vertices for path patterns of $n-1$ length concatenated with $(\elabel_{n}, A_n)$ %$p=\langleA_0, \elabel_1, \cdots, \elabel_{n}, A_n\rangle$ 
is $|\edges(A_n, \elabel_{n})|\cdot {(d_{m})}^{n-1})$ where $n>0$ and $d_{m}$ indicates the maximum in-degrees among vertices.}

\smallskip

{\it Proof}: $|\edges(A_n, \elabel_{n})|$ indicates the number of edges with $\elabel_n$ connecting to vertices whose  attribute set includes $A_n$. Given $\langle A, \elabel_n, A_n \rangle$ as path pattern, the maximum number of vertices that match the path pattern is $|\edges(A_n, \elabel_{n})|$.
When the length of path patterns, the number of paths whose targets' attributes include $A_n$ exponentially increase by $d_m$.
Therefore, the maximum number of matched vertices for path patterns of $n-1$ length concatenated with $(\elabel_{n}, A_n)$ is $|\edges(A_n, \elabel_{n})|\cdot {(d_{m})}^{n-1})$.
\hfill{} $\square$

\smallskip
{\sc Lemma} 3.6. 
{\it Given $A$ and $\elabel$, the maximum number of matched vertices for $\langle A, \elabel, \ldots \rangle$ is $|\vertices(A, \elabel)|$.}

\smallskip

{\it Proof}: This is obvious because the maximum number of vertices that can be sources of paths that match $\langle A, \elabel, \ldots \rangle$ is the number of vertices that have edges with $\elabel$. 
\hfill{} $\square$

\smallskip
{\sc Theorem} 4.1. 
{\it Given frequent path pattern $p$, the missing probability is 
$P\left( \minsup \geq \frac{|\vertices(p)|(d_{m})^{\psi(n-1)}}{p_m(d_p)^{n-1}}{}\right)$, where $p_m$ is a probability that vertex matches with $p$ among paths with the suffix and $d_p$ is the average degree of actual paths.
} 

\smallskip

{\it Proof}: We remove the suffix if $|\edges(A,\elabel)|{(d_{m})^{\psi(n-1)}}$ is not larger than $\minsup$.
We define $|P|$ as the number of paths from any sources to the target of suffix, and $|P| = \vertices(p)\cdot p_m$. Furthermore, $|P| = |\edges(A,\elabel)|(d_p)^{n-1}$.
We can derive the following probability:

\begin{eqnarray}
&P\left( \minsup \geq |\edges(A,\elabel)|{(d_{m})^{\psi(n-1)}}\right)\\
=& P\left( \minsup \geq \frac{|P|}{(d_p)^{n-1}}{(d_{m})^{\psi(n-1)}}\right)\\
=& P\left( \minsup \geq \frac{|\vertices(p)|(d_{m})^{\psi(n-1)}}{p_m(d_p)^{n-1}}{}\right)
\end{eqnarray}
\hfill{} $\square$

\section{Space complexity}
The space complexity of our algorithm is $O(|\vertices|+|\edges|+|\attributes| +|\candidates^A|+|\candidates^S|+|\candidates^*|+|\candidates^R|+\sum_i^k|\pathpatterns_i|+|\pathpatterns^*|+|\rules|)$, where $|\candidates^A|$, $|\candidates^S|$ $|\candidates^*|$, and $|\candidates^R|$ are the maximum sizes of $|\candidates^A_i|$, $|\candidates^S_i|$ $|\candidates^*_i|$, and $|\candidates^R_i|$ for all $i$, respectively.
Generally, the memory space does not become an issue empirically compared with the running time.

\section{Dataset details}

We describe graphs that we used in our experimental studies in detail.
\begin{itemize}
\item Nell~\cite{carlson2010toward} is a knowledge graph crawled from the web.
Its attributes are, for example, ceo, musician, company, and university, and edge labels are, for example, companyceo, competeswith, and workers.
\item DBpedia~\cite{auer2007dbpedia} is a knowledge graph extracted from wikipedia data.
Its attributes are, for example, actor, award, person, and place, and edge labels are, for example, child, spouse, and deathPlace.
%Google+~\cite{gong2012evolution} is a social network owned and operated by Google. 
%Its attributes are, for example, employer, school, major and places, edge label is only follows.
\item Pokec is a social network service in which most users are Slovenian.
Its attributes are, for example, age, gender, city, and music, edge labels are, for example, follows, likes, and locatedIn. The number of edge label follows is very large, so we divide them according to out-degrees, such as small follows and large follows.
\end{itemize}
Table~\ref{table:datasets} shows data statistics.

\begin{table}[t]
\caption{Data statistics.}\label{table:datasets}
  \vspace{-3mm}
\scalebox{0.85}{
\begin{tabular}{lccccc}
\hline
          & $|\vertices|$ & $|\edges|$ & $|\elabels|$ & $|\attributes|$ & Avg. Attr.\\ \hline
Nell      & 46,682      &   231,634     & 821       & 266       & 1.5       \\
DBpedia   & 1,477,796   &   2,920,168   & 504       & 239       & 2.7       \\ 
%Google+   & 909,669   &   47,130,325 & 1            & 991,522   & 4.0       \\ 
Pokec     & 1,666,426   &  34,817,514 & 9            & 36302   & 1.1      \\ 
\hline
\end{tabular}
}
\end{table}

\section{Additional experiment}

We show the impact of length $k$ of paths and approximation factors.

Figure~\ref{fig:runtime_length} shows the run time of each method varying the length $k$.
We set 1,800, 140,000, and 50,000 as $\minsup$.
We do not show the performance of the baseline because it does not finish within 24 hours when $k=3$ in all datasets.
Generally, as length increases, the run time increases because the numbers of rules and path patterns increase.
In Nell, the number of rules drastically increase when $k=4$, our algorithm did not finish within 24 hours.
In DBpedia, the number path patterns does not increase when $k$ is larger than 2, so the run time does not increase.
From these results, we can confirm our approximation methods work well when $k$ is large.

Figure~\ref{fig:runtime_approxiamtiohn} shows the run time varying approximation factor.
The approximation factor indicates candidate reduction $\psi$ factor and sampling rate $\rho$ for CR and SA, respectively.
From this result, we can see that when the approximation factors are small, the run time is small.
However, in Nell, the run time of Our w/ SA is large when $\rho = 0.2$.
This is because the number of false negatives is large, so the frequent rule discovery step takes a large time.

Tables~\ref{table:accuracy_factor_nell}--\ref{table:accuracy_factor_pokec} show the recall and precision varying with approximation factors in each dataset.
We can see that the accuracy are quite high in DBpedia and pokec, while in Nell, CR and SA do not work well when approximation factors are small.
This is because the size of Nell is small compared with DBpedia and pokec, so the candidate reduction and sampling do not work well in some cases.

Table~\ref{table:ablation} shows the run time of our methods that we do not use some techniques.
``Ours w/o suffix pruning'' indicates our method that does not use suffix pruning.
``Ours w/o cost-based parallel'' indicates our method that randomly assigns the same numbers of vertices to threads without considering estimated costs.
From these results, Ours is drastically fast compared with Baseline.
The effectiveness of each technique depends on dataset.
For example, suffix pruning works well in Pokec, while does not in Nell. When the number of attributes is large, the suffix pruning works well.
In parallelization, in Nell and DBpedia, cost-based sampling slightly increase the efficiency, while in Pokec, slightly decreases. In Pokec, the costs of vertices are very similar, so the costs of threads become similar even if we do not estimate their costs. 

\begin{figure*}[!t]
\vspace{-5mm}
  \subfloat[Nell]{\epsfig{file=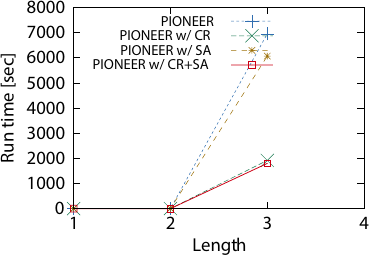,width=0.33\linewidth}
  }
  \subfloat[DBpedia]{\epsfig{file=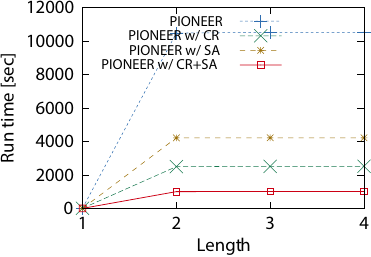,width=0.33\linewidth}
  }
  \subfloat[Pokec]{\epsfig{file=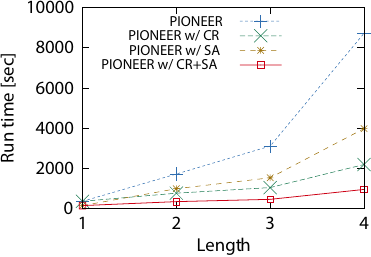,width=0.33\linewidth}
  }
% \subfloat[Index memory]{\epsfig{file=./figures/experiment/k_indexmemory_workload.pdf,width=0.3\linewidth}
%   }
   \vspace{-3mm}
    \caption{Impact of length to run time}
    \label{fig:runtime_length}
\end{figure*}

\begin{figure*}[!t]
\vspace{-5mm}
  \subfloat[Nell]{\epsfig{file=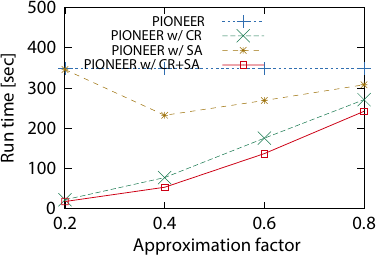,width=0.33\linewidth}
  }
  \subfloat[DBpedia]{\epsfig{file=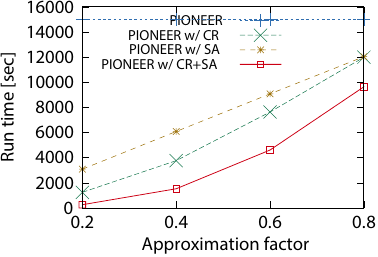,width=0.33\linewidth}
  }
  \subfloat[Pokec]{\epsfig{file=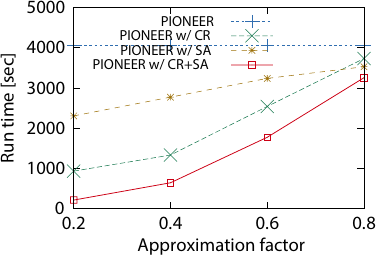,width=0.33\linewidth}
  }
% \subfloat[Index memory]{\epsfig{file=./figures/experiment/k_indexmemory_workload.pdf,width=0.3\linewidth}
%   }
   \vspace{-3mm}
    \caption{Impact of approximation factors to run time}
    \label{fig:runtime_approxiamtiohn}
\end{figure*}

\begin{table}[t]
\caption{Impact of approximation factors to accuracy in Nell}\label{table:accuracy_factor_nell}
   \vspace{-3mm}
\scalebox{0.85}{
\begin{tabular}{l|ll|ll|ll}
\hline
& \multicolumn{2}{|c|}{CR}& \multicolumn{2}{|c|}{SA} & \multicolumn{2}{|c}{CR+SA}\\ 
             & Recall     & Precision & Recall& Precision     & Recall & Precision\\ \hline
0.2	&0.0461	&1	&0.9999	&0.495	&0.046	&0.500\\
0.4	&0.233	&1	&0.9999	&0.999	&0.233	&0.998\\
0.6	&0.532	&1	&0.9999	&0.9999	&0.532	&0.9999\\
0.8	&0.797	&1	&0.9999	&0.9999	&0.797	&0.9999\\

\hline
\end{tabular}
}
\end{table}

\begin{table}[t]
\caption{Impact of approximation factors to accuracy in DBpedia}\label{table:accuracy_factor_dbpedia}
   \vspace{-3mm}
\scalebox{0.85}{
\begin{tabular}{l|ll|ll|ll}
\hline
& \multicolumn{2}{|c|}{CR}& \multicolumn{2}{|c|}{SA} & \multicolumn{2}{|c}{CR+SA}\\ 
             & Recall     & Precision & Recall& Precision     & Recall & Precision\\ \hline
0.2	&1.0	&1.0		&1.0	&1.0	&1.0	&1.0\\
0.4	&1.0	&1.0		&1.0	&1.0	&1.0	&1.0\\
0.6	&1.0	&1.0		&1.0	&1.0	&1.0	&1.0\\
0.8	&1.0	&1.0		&1.0	&1.0	&1.0	&1.0\\
\hline
\end{tabular}
}
\end{table}

\begin{table}[t]
\caption{Impact of approximation factors to accuracy in Pokec}\label{table:accuracy_factor_pokec}
   \vspace{-3mm}
\scalebox{0.85}{
\begin{tabular}{l|ll|ll|ll}
\hline
& \multicolumn{2}{|c|}{CR}& \multicolumn{2}{|c|}{SA} & \multicolumn{2}{|c}{CR+SA}\\ 
             & Recall     & Precision & Recall& Precision     & Recall & Precision\\ \hline
0.2	&1.0	&1.0	&0.934	&0.983	&0.934	&0.983\\
0.4	&1.0	&1.0	&0.967	&0.983	&0.967	&0.983\\
0.6	&1.0	&1.0	&0.984	&0.986	&0.984	&0.984\\
0.8	&1.0	&1.0	&0.984	&0.984	&0.984	&0.984\\
\hline
\end{tabular}
}
\end{table}

\begin{table}
\caption{Ablation study}\label{table:ablation}
  \vspace{-3mm}
\scalebox{0.85}{
\begin{tabular}{l|l|l|l}
\hline
	&Nell	&DBpedia	&Pokec\\\hline
Ours	&341.7	&15028.3	&4038.5\\
Baseline	&525.4	&32907	& ---\\
Ours w/o suffix pruning	&304.4	&15466.4	&6171.3\\
Ours w/o cost-based parallel	&360.4	&15446.8	&4006.9\\
\hline
\end{tabular}
}
\end{table}

\section{Additional related work}

We review studies related to the path association rule mining in four categories; (1) support measure on graphs, (2) association rules, (3) graph pattern mining and matching, and (4) path query.

\begin{table*}[t!]
\caption{Comparison of association rule mining on a single large graph. $\elabels_v$ indicates a set of vertex labels.}\label{table:comparison}
   \vspace{-3mm}
\scalebox{0.85}{
\begin{tabular}{l|lllll}
\hline
                                        &$\graph$& $G_X$ & $G_Y$ & $G_X$ and $G_Y$ &Algorithm\\ \hline
GPAR~\cite{fan2015association}          &$(\vertices, \edges, \elabels, \elabels_v)$& Vertex-centric subgraph & Single edge & $V. G_Y \subseteq V.G_X$ & top-$k$ diverse patterns \\
                                        & &  & (or empty) & & \\ \hline
Extending GPAR~\cite{wang2020extending} &$(\vertices, \edges, \phi, \attributes)$& Subgraph & Subgraph  & $V. G_Y \subseteq V.G_X$ & Frequent patterns\\
                                        & & (at least one edge) &  (at least one edge) & and no common edges  & \\\hline
QGAR~\cite{fan2016adding}               &$(\vertices, \edges, \elabels, \elabels_v)$& Quantified subgraph & Quantified subgraph & $V. G_X \subseteq V.G_Y$ & Application-specific top-$m$ pattern\\\hline
GAR~\cite{fan2022discovering}           &$(\vertices, \edges, \elabels, \attributes)$& Subgraph & single edge or attributes & $V. G_X \subseteq V.G_Y$ & None\\\hline
Ours                                    &$(\vertices, \edges, \elabels, \attributes)$& Path & Path & No restriction & Frequent patterns\\
\hline
\end{tabular}
}
\end{table*}

{\bf Graph association rule mining. }
We show the semantics of each graph association rule mining in Table~\ref{table:comparison}.

\smallskip
\noindent
{\bf Graph pattern mining and matching.}
A number of algorithms have been developed for graph pattern matching~
\cite{elseidy2014grami, shelokar2014three}. %ke2009efficient
Graph pattern mining algorithms possibly accelerate discovering graph association rules.
Similarly, algorithms for isomorphic subgraph matching, e.g., \cite{han2019efficient,fan2020extending},
%lee2012depth
are developed for efficiently discovering matched patterns in a single large graph.
These methods are not suitable for discovering frequent path patterns because they require to find subgraphs from scratch repeatedly.
Our algorithm maintains the targets of paths to efficiently extend the path patterns and uses anti-monotonic properties to reduce the number of candidates.
In addition, graph pattern mining and matching techniques do not handle reachability path patterns.

\smallskip
\noindent
{\bf Path query.}
The path association rule aims to discover regularities between paths instead of subgraphs.
Querying path patterns are actively studied due to their usefulness~\cite{AnglesABHRV17,AnglesRV19}.
%Current practical languages on graph databases such as SPARQL~\cite{perez2006semantics}, Cypher~\cite{cypher}, PGQL~\cite{van2016pgql}, and GSQL~\cite{gsql}, G-CORE~\cite{angles2018g}, and SQL/PGQ \cite{sqlpg}, are based on the abilities for querying complex path and graph patterns.
In recent real-life query logs for Wikidata~\cite{vrandevcic2014wikidata}, more than 90 \% of queries are path patterns~\cite{bonifati2020analytical,BonifatiMT19}.
From this fact, graph analysis often utilizes path patterns instead of graph patterns to understand real-world relationships.
Therefore, path association rule mining can be useful in real-world analysis on many applications.

\bibliographystyle{ACM-Reference-Format}
\bibliography{graphassociationrule}

% \newpage

% \section*{Appendix}

% \begin{theorem}\label{theo:dominate}
% If path pattern $p \subseteq p'$, $\vertices(p) \supseteq \vertices(p')$.
% \end{theorem}
% {\it Proof}: When $p$ is dominated by $p'$, $p$ is not longer than $p'$, all edge labels on $p$ and $p'$ are the same order, and attribute sets on $p$ are subset or equal to those on $p'$.
% All vertices that match $p'$ are matched with path patterns whose attributes are subset of $p'$.
% Therefore, if path pattern $p \subseteq p'$, $\vertices(p) \supseteq \vertices(p')$.
% \hfill{} $\square$

% \begin{lemma}\label{lemma:antimonotonicity_1}
% If prefix of path patterns is not frequent, the whole path patterns are not frequent.
% \end{lemma}
% {\it Proof}: If $v$ matches $p=(A_0, \elabel_1, \cdots, \elabel_{n}, A_m)$, $v$ matches $(A_0, \elabel_1, \cdots,$ $\elabel_{n}, A_m)$ where $m < n$.
% Similarly, if  $v$ does note match $(A_0, \elabel_1, \cdots,$ $\elabel_{m}, A_m)$, $v$ does not matches $(A_0, \elabel_1, \cdots, \elabel_{n}, A_n)$.
% Therefore, if prefix of path patterns is not frequent, the whole path patterns are not frequent.
% \hfill{} $\square$

% \begin{lemma}\label{lemma:antimonotonicity_2}
% If path pattern $p$ is not frequent, $p'$ such that $\forall A_i' \supseteq A_i$ and $\elabel_i = \elabel'_i$ is not frequent.
% \end{lemma}
% \noindent
% {\it Proof}: If $v$ matches $p'$, $v$ matches $p$ because $p'$ is more complex than $p$.
% Similarly, if  $v$ does note match $p$, $v$ does not matches $p'$.
% Therefore, if $p$ is not frequent, $p'$ is not frequent.
% \hfill{} $\square$

\end{document}
